# Supplementary material for: Fractal energy spectrum of a polariton gas in a Fibonacci quasi-periodic potential
Source: arXiv:1311.3453 source file (2014-02-24)
Supplement: Supplementary file 1 [file SuppMat.pdf]

# Supplementary material for "Fractal energy spectrum of a polariton gas in a Fibonacci quasi-periodic potential"

D. Tanese[1], E. Gurevich[2], F. Baboux[1], T. Jacqmin[1], A. Lemaître[1],
E. Galopin[1], I. Sagnes[1], A. Amo[1], J. Bloch[1], E. Akkermans[2]
[1]*Laboratoire de Photonique et de Nanostructures, LPN/CNRS, Route de Nozay, 91460 Marcoussis, France and*
[2]*Department of Physics, Technion Israel Institute of Technology, Haifa 32000, Israel*
(Dated: February 24, 2014)

In this Supplementary Material, we present additional experimental data supporting our claim about fractal properties of the Fibonacci spectrum and in particular the invariance of the IDOS in the gaps in accordance with the gap labeling theorem (7) discussed in the Letter. We then present a brief but explicit derivation of the 1D Schrödinger equation with the effective potential $V(x)$ given by equation (4) of the Letter. We stress the importance of the second, often omitted, term in $V(x)$ and then compare the results obtained within this effective 1D approach to those obtained using a full fledged numerical calculation of the 2D polariton spectrum.

## EXPERIMENTAL ILLUSTRATION OF THE TOPOLOGICAL INVARIANCE OF THE IDOS

In order to illustrate the topological invariance of the integrated density of states (IDOS) measured on a polariton gas laterally confined by a Fibonacci potential, we describe here additional data obtained for different system sizes and realizations of the potential. The results are presented in a similar way as in the paper so that they can be directly compared to Figs. 3 and 4. These new data confirm that the wave vector values at which the mini-gaps open in the Fibonacci spectrum, as well as the corresponding values of the IDOS, are invariant quantities of topological nature, *i.e.* that they do not depend on the specific shape of the quasi-periodic potential felt by the polaritons nor on the size of the letters.

We study two additional samples (hereafter called samples 2 and 3 by contrast to sample 1 which corresponds to the one presented in the Letter). These samples have a different length $a$ of the letters than sample 1 (which had $a = 0.8$ $\mu$m). Sample 2 has longer letters ($a = 1.35$ $\mu$m), while sample 3 has shorter ones ($a = 0.5$ $\mu$m). Furthermore, while sample 3 has letter widths identical to those of sample 1 ($w_A = 3.5$ $\mu$m and $w_B = 1.86$ $\mu$m), sample 2 has a different $w_B = 2.04$ $\mu$m, which results in a smaller potential contrast between the two types of letters. Moreover samples 2 and 3 also differ from sample 1 by their total number of letters, and thus correspond to different orders of the Fibonacci sequence: $S_{12}$ (144 letters) for sample 2, $S_{14}$ (377 letters) for sample 3, as compared to $S_{13}$ (233 letters) for sample 1.

Figures 1 and 2 display the spectrally resolved far field emission, the density of states (DOS) and the IDOS measured on samples 2 and 3, together with corresponding calculations.

Let us first discuss the far field emission shown in the top panels of the two figures. As in Fig. 3 of the Letter, mini-gaps open, whose positions in momentum space can be accurately labeled (see arrows) by means of two integers $[p, q]$ such that $k = \frac{\pi}{a}(p + q\sigma^{-1})$, in accordance with the gap labeling theorem (7). Comparing these spectra with sample 1 allows to understand their scaling properties. Since the momentum $k$-positions of the gaps scale as $\frac{\pi}{a}$, the spectrum of sample 2 appears "compressed" in energy with respect to that of sample 1: for instance, the gap $[-1, 2]$ appears much closer to the bottom of the parabola. Thus, due to the finite polariton linewidth, only one mode is visible below this gap (instead of three for sample 1 in the Letter). For sample 3 instead, the spectrum appears "stretched" with respect to sample 1, and more modes and mini-gaps can be experimentally identified below this $[-1, 2]$ gap than in the Letter.

The values of the IDOS in the mini-gaps are also invariant topological quantities. This is illustrated in Figs. 1(d) and 2(d) where the theoretical values $\mathcal{N}(E_{Q_{p,q}/2}) = p + q\sigma^{-1}$ for the IDOS inside the gaps (see Eq. (7) of the Letter), predicted by the gap labeling theorem, are indicated with red horizontal arrows. Both numerical and experimental results reproduce well the values of the heights of the plateaus.

To conclude, the overall data presented in our work provides a solid illustration of the scaling properties of the gaps positions and topological invariance of the IDOS, as ensured by the gap labeling theorem (7).

## DERIVATION OF THE EXPRESSION OF THE EFFECTIVE POTENTIAL GIVEN BY EQUATION (4)

We now turn to the derivation and discussion of the validity of the 1D Schrödinger equation with the effective potential $V(x)$,

$$V(x) = \frac{\pi^2}{w^2(x)} + \frac{\pi^2 + 3}{12}\left(\frac{w'(x)}{w(x)}\right)^2 \qquad (1)$$

given by Eq. (4) in the Letter. To that aim, we need to map the original 3D setup onto an effective 1D prob-

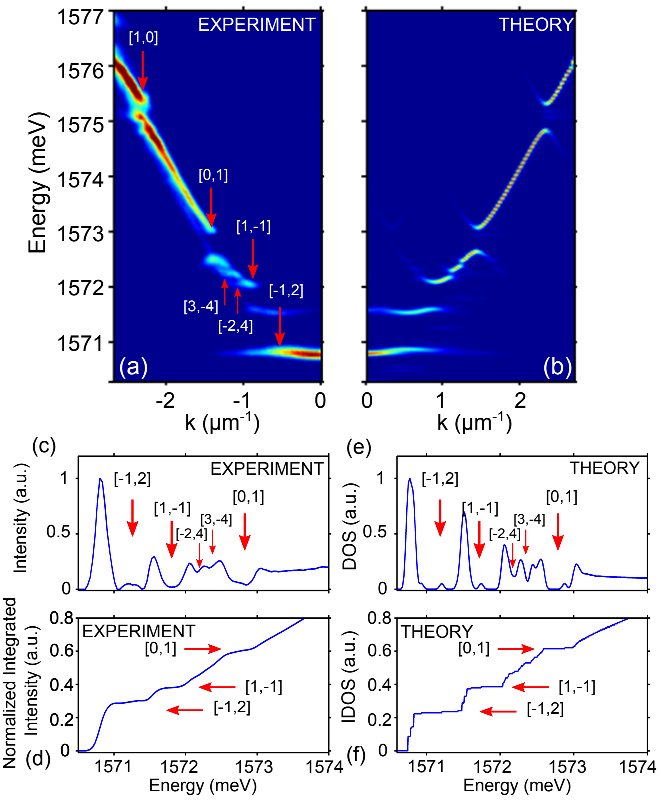


FIG. 1: (Color online) (a) Spectrally resolved far field emission measured on sample 2 (parameters given in the text) and (b) corresponding numerical results obtained with the effective 1D model described in the Letter and in the next section. The positions of the gaps are labeled with two integers $[p, q]$ and indicated with red arrows. (c) Measured total (angular-averaged) emission spectrum $I(\varepsilon)$ and (d) normalized integrated emission intensity $\int_{E_0}^{\varepsilon} I(\varepsilon')d\varepsilon'$ (with $E_0$ the lower energy state). (e) Calculated DOS smoothed for the comparison with $I(\varepsilon)$ in (c). (f) Normalized calculated IDOS.

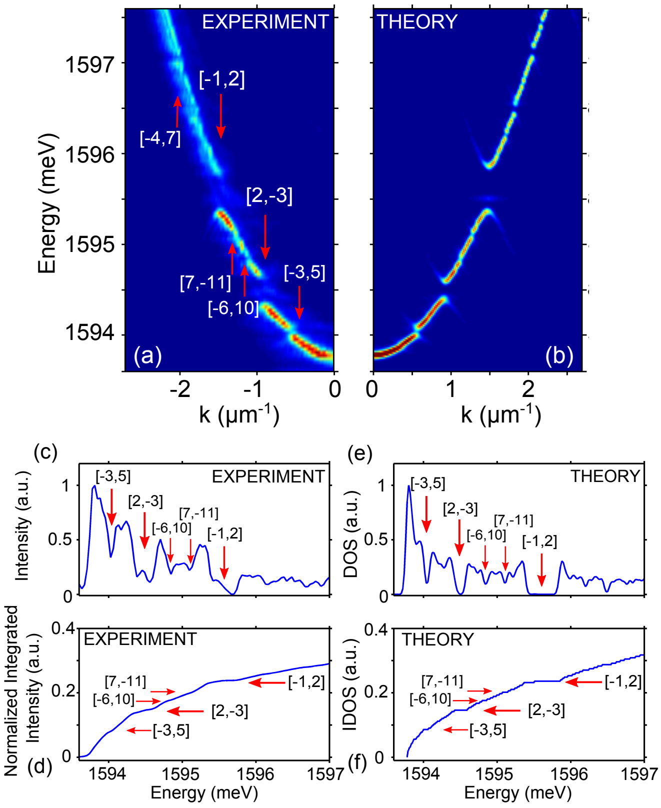


FIG. 2: (Color online) Same as Fig. 1 for sample 3 (parameters in the text).

lem. As described in more detail in the Letter, polaritonic wires are fabricated by processing a planar $\lambda/2$ cavity. We denote $n$ its effective refractive index. The electromagnetic field is confined along the (vertical) $z$-direction using two Bragg mirrors. This confinement is much tighter than that in the perpendicular $xy$-plane. For the latter, we impose zero boundary conditions, an approximation justified by the high contrast in refractive index between dielectric and air (see, e.g., Ref. [1]). Under the above assumptions, the corresponding electromagnetic field eigenmodes can be chosen to have either TE or TM polarizations. The polarization splitting is large in an etched wire cavity, probably because of strain relaxation. Since in the experiment we detect only one polarization, we do not include the polarization degree of freedom in the simulation and we consider a scalar wave approximation. Then, looking for separable solutions between vertical and lateral coordinates, leads to the following two-dimensional (2D) stationary wave equation

$$E\psi(x,y) = -\frac{\hbar^2}{2m_{ph}}\triangle_\perp \psi(x,y)\,, \tag{2}$$

where $m_{ph} \equiv n^2 E_c/c^2$ is the effective photon mass, $E_c \equiv \frac{\hbar c}{n} k_z$ is the energy associated with the fundamental mode of the $\lambda/2$ cavity, and $\triangle_\perp \equiv \partial_x^2 + \partial_y^2$ is the transverse Laplacian. Since $E \ll E_c$, the total photon energy can be expanded in $E$ so that,

$$\hbar\omega \approx E_c + E\ . \tag{3}$$

As a result of our assumed zero boundary conditions in the $xy$-plane, the electromagnetic field $\psi(x,y)$ vanishes on the boundary.

Note that Eq.(2), with the same boundary conditions, also holds to describe the center-of-mass motion of the excitons confined to the $xy$-plane by the quantum wells. Therefore, within the same approximations, the electromagnetic field and the excitons have similar eigenmodes and energy spectrum (up to the difference in their effective mass), so that the photon-exciton coupling is diagonal in the eigenmode index. A flat exciton dispersion is used because of their relatively large mass. The finding of the eigenmodes of the 2D problem (2) on a strip can easily be done numerically. Nevertheless, it is useful to have

a well controlled 1D effective model providing intuition and insight of the essential features of the problem at hand. This is particularly relevant for the quasi-periodic potential we study and its fractal polariton spectrum, since a broad range of analytical and numerical tools are specifically available for the 1D problem, such as the gap labeling theorem used in the Letter.

To proceed further and establish the expression of the 1D effective potential Eq.(1), we look for solutions of the wave equation Eq. (2) on a symmetric strip defined by its longitudinal coordinate $x \in [0, L]$, where $L$ is the length of the wire, and its transverse coordinate $-\frac{w(x)}{2} \leq y \leq \frac{w(x)}{2}$. The function $w(x) > 0$, which defines the $x$-dependent width of the wire, is assumed to be differentiable. The sought solution can generally be written in the form of a Fourier series over the transverse quasi-modes,

$$\psi(x, y) = \sum_{n=0}^{\infty} \psi_n(x) \sqrt{\frac{2}{w(x)}} \cos(k_{y,n}(x)\, y), \qquad (4)$$

where both the transverse wave vector, $k_{y,n}(x) = \pi \frac{2n+1}{w(x)}$, and the expansion coefficients $\psi_n(x)$, are $x$-dependent. This solution is symmetric with respect to the middle line $y = 0$, and it is not coupled to the similar anti-symmetric one (note that for a non-symmetric strip, both solutions would participate to the expansion (4)). We need to consider only symmetric solutions, since they include the lowest frequency branch, corresponding to the lowest transverse quasi-mode, $k_{y,0}(x) = \frac{\pi}{w(x)}$. An infinite hierarchy of coupled differential equations for $\psi_m(x)$ is obtained by substituting the expansion (4) into the wave equation (2) and subsequently integrating over $y$ with the weight $\sqrt{\frac{2}{w(x)}} \cos(k_{y,m}(x)\, y)$. Neglecting the coupling to the higher quasi-modes, leads to the following approximate equation for the lowest quasi-mode:

$$E\psi_0(x) = \frac{\hbar^2}{2m_{ph}} \left[ -\frac{d^2}{dx^2} + V(x) \right] \psi_0(x), \qquad (5)$$

where $V(x)$ given in Eq.(1), defines the effective 1D potential along the strip for the lowest transverse mode. Similar results have been obtained for the study of cold atoms in optical trap waveguides [2]. The coupling of $\psi_0(x)$ to the higher quasi-modes leads to the appearance of additional terms in Eq.(5), involving various derivatives of $w(x)$. For a coupling strength between quasi-modes small compared to the energy separation to the next mode, we can neglect those additional terms. The detailed analysis of this conditions is, however, beyond the scope of this supplement. Instead, we justify this approximation comparing our results to the full fledged 2D numerics.

The first term in the potential $V(x)$ given in Eq.(1) is the usual adiabatic approximation, proportional to $k_{y,0}^2(x)$, which accounts for the distribution of the "kinetic" energy between the transversal and the longitudinal degrees of freedom. For a constant $w(x)$, the problem is separable. It leads to uncoupled transverse modes $\psi_m(x)$ and the adiabatic kinetic term is the only remaining contribution to $V(x)$. For a varying profile $w(x)$ such as the one we consider, the problem is not separable anymore, and the second term in Eq.(1) becomes relevant. This term is sensitive to the stiffness of the boundary variation [2]. For a smoothly varying width, $w'(x)$ is small and the second term is negligible compared to the kinetic term. For a sharper step structure, like the one we consider (see Fig. 1(b)-(c) of the Letter), the two terms in the effective potential become comparable. In the limit in of sharp steps for $V(x)$, the second term in Eq.(1) becomes singular, namely a repulsive $\delta$-function squared. In that case, higher transversal quasi-modes must be included.

## COMPARISON BETWEEN THE EXACT 2D CALCULATION AND THE EFFECTIVE 1D POTENTIAL

We wish now to show that the effective 1D model provides a quantitatively good description of the measured polariton spectrum provided we include the second term in the potential (1) which account for the sharp boundary modulation. To that purpose, we compare the low energy eigenmode spectra obtained from the exact two-dimensional (2D) and the effective one-dimensional calculations. The 2D calculation is done using, instead of (4), a complete two-dimensional Fourier expansion, and then diagonalizing the Hamiltonian in this two-dimensional basis. In addition, a scale is introduced over which we smoothen the width profile by means of a convolution of the binary width profile with the Gaussian kernel,

$$g(x) \propto e^{-(x/\eta a)^2}, \qquad (6)$$

where $a$ is the letter length and the relative dimensionless smoothness scale $\eta$ is used as a fitting parameter (to the experimental data). This is justified looking at the micrograph of the wire in Fig. 1(b) of the Letter. Obviously, there is some smoothness in the wire width variation, introduced by the etching process. Its scale, however, is hard to quantify from the direct measurement, and should be considered as a phenomenological parameter. In order to compare the effective 1D description to the full 2D calculation, we consider sample 2 described above ($a = 1.35\ \mu$m), and plot in Fig. 3 the integrated density of states (IDOS) for different values of the fitting parameter $\eta$. We note that the position and the width of the gaps of the 2D spectrum are significantly less sensitive to the parameter $\eta$ than the effective 1D spectrum. Note

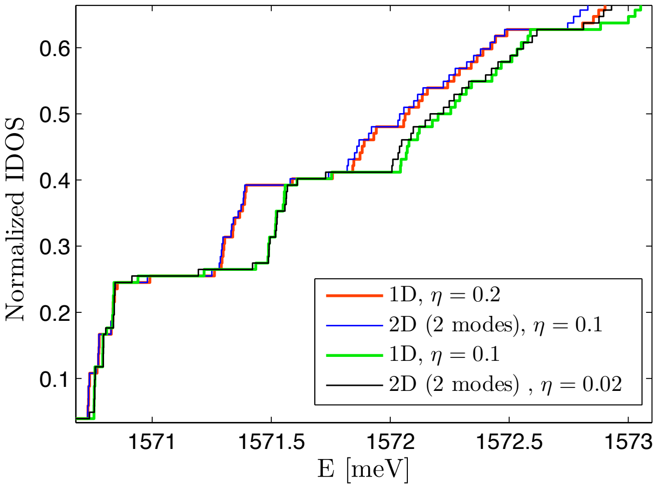


FIG. 3: (Color online) Comparison, for sample 2, between the results obtained for the IDOS based on the full 2D and the 1D calculations using the effective potential $V(x)$ given by Eq. (1). The values of smoothing parameter $\eta$ are indicated in the inset.

however, that the value of the IDOS in the gaps is independent of $\eta$ in both cases, since it is a topologically stable quantity. These different sensitivities to the parameter $\eta$ can be rather exactly compensated by increasing the smoothness scale in the 1D calculation relatively to the corresponding 2D case. This is demonstrated in Fig. 3 by superimposing the two results for different sets of choices of $\eta$. On the other hand, the 1D calculation using only the first (kinetic) term in $V(x)$ does not show any specific dependence on $\eta$ even for rather large values of the smoothing. It is thus not possible to use this approximation to reproduce the 2D calculation. Moreover, the 1D potential based on the first kinetic term only in Eq.(1), is unable to reproduce the gap structure of the spectrum, even qualitatively. To show this, we have plotted in the left panel of Fig. 4, the spectral function of the 2D calculation. It is compared (right panel) to the 1D spectral function obtained using the first term only in Eq. (1). We note the discrepancy in the position of the gaps which cannot be handled by a proper choice of $\eta$. More important, the higher energy gaps (*e.g.* the one labeled $[1, 0]$) in Fig. 3 of the Letter are missing. In contrast, the full 1D effective model with a proper value of $\eta$ reproduces faithfully both the 2D and the measured spectra.

[1] A. Kuther, M. Bayer, T. Gutbrod, A. Forchel, P. A. Knipp, T. L. Reinecke, and R. Werner, Phys. Rev. B **58**, 15744 (1998).

[2] S Schwartz, M Cozzini, C Menotti, I Carusotto, P Bouyer and S Stringari, New Journal of Physics **8**, 162 (2006).

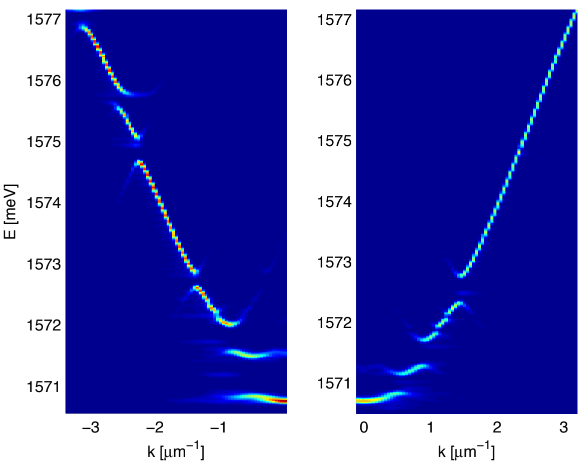


FIG. 4: (Color online) Comparison, for sample 2, between the spectral function obtained from the full 2D calculation (left) versus the 1D calculation using the effective potential $V(x)$ given by Eq.(1) where only the first kinetic term has been considered (right).
